# Supplementary material for: Feature Decomposition for Reducing Negative Transfer: A Novel Multi-task Learning Method for Recommender System
Source: arXiv:2302.05031 source file (2023-02-10)
Supplement: Supplementary file 1 [file appendix.tex]

\section{Appendix}
\subsection{Synthetic Data Generation}
Synthetic data generation steps as follow:
\begin{itemize}
\item [1)]
Randomly generated unit vector $u_{1}, u_{2}, u_{s} \in R^{d}$ :
\begin{equation}
\left\|u_{1}\right\|_{2}=1,\left\|u_{2}\right\|_{2}=1,\left\|u_{s}\right\|_{2}=1
\end{equation}

\item [2)]
Given constant $c_{1}, c_{2}, c_{s}$ generate weight vector:
\begin{equation}
w_{1}=c_{1} u_{1}, w_{2}=c_{2} u_{2}, w_{s}=c_{s} u_{s}
\end{equation}

\item [3)]
Randomly generated $x_{1}, x_{2}, x_{s} \in R^{d}$, where $x_{1}^{i} \sim N(-1,0.1), x_{2}^{i} \sim N(1,0.1), x_{s}^{i} \sim N(0,1)$.

\item [4)]
Generate two labels for regression tasks:
\begin{equation}
y_{1}=s+w_{1}^{T} x_{1}+\sum_{i=1}^{m} \sin \left(\alpha_{i} w_{1}^{T} x_{1}+\beta_{i}\right)+\epsilon_{1}
\end{equation}
\begin{equation}
y_{2}=s+w_{2}^{T} x_{2}+\sum_{i=1}^{m} \sin \left(\alpha_{i} w_{2}^{T} x_{2}+\beta_{i}\right)+\epsilon_{2}
\end{equation}
where $s=w_{s}^{T} x_{s}+\sum_{i=1}^{m} \sin \left(\alpha_{i} w_{s}^{T} x_{s}+\beta_{i}\right), \epsilon_{1}, \epsilon_{2} \stackrel{\text { i.i.d }}{\sim} N(0,0.01)$

\item [5)]
Generate features:
\begin{equation}
\begin{aligned}
X_{1 i}=& \sin \left(\delta_{i}\left(u_{1}^{i} x_{1}^{i}+u_{s}^{i} x_{s}^{i}\right)+\gamma_{i}\right) + \\ & \cos \left(\delta_{i}\left(u_{1}^{i} x_{1}^{i}+u_{s}^{i} x_{s}^{i}\right)+\gamma_{i}\right)+\varepsilon
\end{aligned}
\end{equation}
\begin{equation}
\begin{aligned}
X_{2 i}=& \sin \left(\delta_{i}\left(u_{2}^{i} x_{2}^{i}+u_{s}^{i} x_{s}^{i}\right)+\gamma_{i}\right)+ \\ & \cos \left(\delta_{i}\left(u_{2}^{i} x_{2}^{i}+u_{s}^{i} x_{s}^{i}\right)+\gamma_{i}\right)+\varepsilon
\end{aligned}
\end{equation}
\begin{equation}
\begin{aligned}
X_{i}=&\sin \left(\delta_{i}\left(u_{1}^{i} x_{1}^{i}+u_{2}^{i} x_{2}^{i}+u_{s}^{i} x_{s}^{i}\right)+\gamma_{i}\right)+ \\ & \cos \left(\delta_{i}\left(u_{1}^{i} x_{1}^{i}+u_{2}^{i} x_{2}^{i}+u_{s}^{i} x_{s}^{i}\right)+\gamma_{i}\right)+\varepsilon
\end{aligned}
\end{equation}
where $\varepsilon \stackrel{\text { i.i.d }}{\sim} N(0,0.01)$ , $X_{1 i}$ and $X_{2 i}$ as a feature of the single task model, $X_{i}$ as a feature of multitasking dataset.

\item [6)]
Repeat 3), 4) and 5) until enough data are generated.
\end{itemize}
